# Supplementary material for: Learning Linear Temporal Properties from Noisy Data: A MaxSAT Approach
Source: arXiv:2104.15083 source file (2021-06-24)
Supplement: Supplementary file 1 [file appendix.tex]

\clearpage
\appendix

\section{More comparison between tested algorithms}
\label{app:sec:evaluation}

% !TEX root = main.tex

\FloatBarrier
\subsection{\MaxSAT{} compared to \SAT{}}

We compare \MaxSAT{} (proposed in this paper) and \SAT{} (proposed in \cite{DBLP:conf/fmcad/NeiderG18})
in Figures \ref{app:fig:sat-vs-maxsat:time} and \ref{app:fig:sat-vs-maxsat:LTL}.

\begin{figure*}[h]
\centering
\vspace{-4mm}
\begin{subfigure}{.4\linewidth}
	\centering
	\includepgfgenerate[fig-app-eval-11a.tex]{
		loglog
		--title 'Benchmark without noise'
		--xlabel '\SAT{} ($s$)' --ylabel '\MaxSAT{}($\thres=0.00$) ($s$)'
		--table joinedByTraces.csv
		--keep-only benchmark_noise:0.0
		--columns runtime_SAT:runtime_MaxSAT0
	}
\end{subfigure}
%\hspace{1.5cm}
\begin{subfigure}{.4\linewidth}
	\centering
	\includepgfgenerate[fig-app-eval-11b.tex]{
		loglog
		--title 'Benchmark with 5\% noise'
		--xlabel '\SAT{} ($s$)' --ylabel '\MaxSAT{}($\thres=0.00$) ($s$)'
		--table joinedByTraces.csv
		--keep-only benchmark_noise:0.05
		--columns runtime_SAT:runtime_MaxSAT0
	}
\end{subfigure}

\begin{subfigure}{.4\linewidth}
	\centering
	\includepgfgenerate[fig-app-eval-11c.tex]{
		loglog
		--title 'Benchmark without noise'
		--xlabel '\SAT{} ($s$)' --ylabel '\MaxSAT{}($\thres=0.05$) ($s$)'
		--table joinedByTraces.csv
		--keep-only benchmark_noise:0.0
		--columns runtime_SAT:runtime_MaxSAT5
	}
\end{subfigure}
%\hspace{1.5cm}
\begin{subfigure}{.4\linewidth}
	\centering
	\includepgfgenerate[fig-app-eval-11d.tex]{
		loglog
		--title 'Benchmark with 5\% noise'
		--xlabel '\SAT{} ($s$)' --ylabel '\MaxSAT{}($\thres=0.05$) ($s$)'
		--table joinedByTraces.csv
		--keep-only benchmark_noise:0.05
		--columns runtime_SAT:runtime_MaxSAT5
	}
\end{subfigure}

\begin{subfigure}{.4\linewidth}
	\centering
	\includepgfgenerate[fig-app-eval-11e.tex]{
		loglog
		--title 'Benchmark without noise'
		--xlabel '\SAT{} ($s$)' --ylabel '\MaxSAT{}($\thres=0.10$) ($s$)'
		--table joinedByTraces.csv
		--keep-only benchmark_noise:0.0
		--columns runtime_SAT:runtime_MaxSAT10
	}
\end{subfigure}
%\hspace{1.5cm}
\begin{subfigure}{.4\linewidth}
	\centering
	\includepgfgenerate[fig-app-eval-11f.tex]{
		loglog
		--title 'Benchmark with 5\% noise'
		--xlabel '\SAT{} ($s$)' --ylabel '\MaxSAT{}($\thres=0.10$) ($s$)'
		--table joinedByTraces.csv
		--keep-only benchmark_noise:0.05
		--columns runtime_SAT:runtime_MaxSAT10
	}
\end{subfigure}

\caption{
	Running time comparison in seconds of \SAT{} and \MaxSAT{}
	with different values for the threshold $\thres$.
	$900 s$ of running time means that the algorithm timed out.
}
\label{app:fig:sat-vs-maxsat:time}
\vspace{-11mm}
\end{figure*}

\begin{figure*}[h]
\centering

\begin{subfigure}{0.45\linewidth}
	\centering
	\includepgfgenerate[fig-app-eval-12a.tex]{
		bubble
		--title 'Benchmark without noise'
		--xlabel '\SAT{}' --ylabel '\MaxSAT{}($\thres=0.00$)'
		--table SizeFreq-MaxSATvsSAT-timeouts.csv
		--columns SAT-perf1:MaxSAT0-perf:Freq-perf1
	}
\end{subfigure}
\begin{subfigure}{0.45\linewidth}
	\centering
	\includepgfgenerate[fig-app-eval-12b.tex]{
		bubble
		--title 'Benchmark with 5\% noise'
		--xlabel '\SAT{}' --ylabel '\MaxSAT{}($\thres=0.00$)'
		--table SizeFreq-MaxSATvsSAT-timeouts.csv
		--columns SAT-noisy1:MaxSAT0-noisy:Freq-noisy1
	}
\end{subfigure}

\begin{subfigure}{0.45\linewidth}
	\centering
	\includepgfgenerate[fig-app-eval-12c.tex]{
		bubble
		--title 'Benchmark without noise'
		--xlabel '\SAT{}' --ylabel '\MaxSAT{}($\thres=0.05$)'
		--table SizeFreq-MaxSATvsSAT-timeouts.csv
		--columns SAT-perf2:MaxSAT5-perf:Freq-perf2
	}
\end{subfigure}
\begin{subfigure}{0.45\linewidth}
	\centering
	\includepgfgenerate[fig-app-eval-12d.tex]{
		bubble
		--title 'Benchmark with 5\% noise'
		--xlabel '\SAT{}' --ylabel '\MaxSAT{}($\thres=0.05$)'
		--table SizeFreq-MaxSATvsSAT-timeouts.csv
		--columns SAT-noisy2:MaxSAT5-noisy:Freq-noisy2
	}
\end{subfigure}

\begin{subfigure}{0.45\linewidth}
	\centering
	\includepgfgenerate[fig-app-eval-12e.tex]{
		bubble
		--title 'Benchmark without noise'
		--xlabel '\SAT{}' --ylabel '\MaxSAT{}($\thres=0.10$)'
		--table SizeFreq-MaxSATvsSAT-timeouts.csv
		--columns SAT-perf3:MaxSAT10-perf:Freq-perf3
	}
\end{subfigure}
\begin{subfigure}{0.45\linewidth}
	\centering
	\includepgfgenerate[fig-app-eval-12f.tex]{
		bubble
		--title 'Benchmark with 5\% noise'
		--xlabel '\SAT{}' --ylabel '\MaxSAT{}($\thres=0.10$)'
		--table SizeFreq-MaxSATvsSAT-timeouts.csv
		--columns SAT-noisy3:MaxSAT10-noisy:Freq-noisy3
	}
\end{subfigure}

\caption{
	Inferred \LTLf{} formula size comparison of \SAT{} and \MaxSAT{}
	with different values for the threshold $\thres$.
	The surface of the dots is proportional to the number of samples represented.
	We denote \LTLf{} formula not inferred because of timeouts by $\emptyset$.
}
\label{app:fig:sat-vs-maxsat:LTL}
\end{figure*}

\FloatBarrier
\subsection{\MaxSATDT{} compared to \MaxSAT{}}

We compare \MaxSATDT{} to \MaxSAT{} (both proposed in this paper) in Figure \ref{app:fig:maxsat-vs-maxsatdt}.

\begin{figure*}[h]
\centering
\begin{subfigure}{.45\linewidth}
	\centering
	\includepgfgenerate[fig-app-eval-21a.tex]{
		loglog
		--title 'Running time in $s$'
		--xlabel '\MaxSAT{}' --ylabel '\MaxSATDT{}($\minscore=0.80$)'
		--table joinedByTraces.csv
		--columns runtime_MaxSAT5:runtime_MaxSATDT80
		--min=1e-3 %--max=1e3
	}
\end{subfigure}
%\hspace{1.5cm}
\begin{subfigure}{.45\linewidth}
	\centering
	\includepgfgenerate[fig-app-eval-21b.tex]{
		loglog
		--title 'Inferred \LTLf{} formula size'
		--xlabel '\MaxSAT{}' --ylabel '\MaxSATDT{}($\minscore=0.80$)'
		--table joinedByTraces.csv
		--columns LTL_size_MaxSAT5:LTL_size_MaxSATDT80
		--min=1 --max=250
	}
\end{subfigure}

\begin{subfigure}{.45\linewidth}
	\centering
	\includepgfgenerate[fig-app-eval-21c.tex]{
		loglog
		--title 'Running time in $s$'
		--xlabel '\MaxSAT{}' --ylabel '\MaxSATDT{}($\minscore=0.60$)'
		--table joinedByTraces.csv
		--columns runtime_MaxSAT5:runtime_MaxSATDT60
		--min=1e-3 %--max=1e3
	}
\end{subfigure}
%\hspace{1.5cm}
\begin{subfigure}{.45\linewidth}
	\centering
	\includepgfgenerate[fig-app-eval-21d.tex]{
		loglog
		--title 'Inferred \LTLf{} formula size'
		--xlabel '\MaxSAT{}' --ylabel '\MaxSATDT{}($\minscore=0.60$)'
		--table joinedByTraces.csv
		--columns LTL_size_MaxSAT5:LTL_size_MaxSATDT60
		--min=1 --max=250
	}
\end{subfigure}

\caption{
	Comparison on all benchmarks of the performances of \MaxSATDT{}($\minscore$) and \MaxSAT{},
	with $\thres=0.05$ for both algorithms.
	$900 s$ of running time means that the algorithm timed out.
}
\label{app:fig:maxsat-vs-maxsatdt}
\end{figure*}

\clearpage
\FloatBarrier
\subsection{\MaxSATDT{} performances in function of $\minscore$ parameter}

We evaluate the effects of $\minscore$ parameter on \MaxSATDT{} (proposed in this paper)
in Figure \ref{app:fig:maxsatdt}

\begin{figure*}[h]
\centering
\begin{subfigure}{.45\linewidth}
	\centering
	\includepgfgenerate[fig-app-eval-31a.tex]{
		loglog
		--title 'Running time in $s$'
		--xlabel '\MaxSATDT{}($\minscore=0.80$' --ylabel '\MaxSATDT{}($\minscore=0.60$)'
		--table joinedByTraces.csv
		--columns runtime_MaxSATDT80:runtime_MaxSATDT60
		--min=1e-3 %--max=1e3
	}
\end{subfigure}
%\hspace{1.5cm}
\begin{subfigure}{.45\linewidth}
	\centering
	\includepgfgenerate[fig-app-eval-31b.tex]{
		loglog
		--title 'Inferred \LTLf{} formula size'
		--xlabel '\MaxSATDT{}($\minscore=0.80$' --ylabel '\MaxSATDT{}($\minscore=0.60$)'
		--table joinedByTraces.csv
		--columns LTL_size_MaxSATDT80:LTL_size_MaxSATDT60
		--min=1 --max=250
	}
\end{subfigure}

\caption{
	Comparison on all benchmarks of the performances of \MaxSATDT{}($\minscore$)
	with respectively $\minscore=0.80$ and $\minscore=0.60$.
	$\thres$ is set to $0.05$.
	$900 s$ of running time means that the algorithm timed out.
}
\label{app:fig:maxsatdt}
\end{figure*}

\clearpage
\FloatBarrier
\subsection{\MaxSATDT{} compared to \SATDT{}}

We compare \MaxSATDT{} (proposed in this paper) and \SATDT{} (proposed in \cite{DBLP:conf/fmcad/NeiderG18})
in Figure \ref{app:fig:satdt-vs-maxsatdt}.

\begin{figure*}[h]
\centering
\begin{subfigure}{.45\linewidth}
	\centering
	\includepgfgenerate[fig-app-eval-41a.tex]{
		loglog
		--title 'Running time in $s$'
		--xlabel '\SATDT{}' --ylabel '\MaxSATDT{}($\minscore=0.80$)'
		--table joinedByTraces.csv
		--columns runtime_SATDT:runtime_MaxSATDT80
		--min=1e-3 %--max=1e3
	}
\end{subfigure}
%\hspace{1.5cm}
\begin{subfigure}{.45\linewidth}
	\centering
	\includepgfgenerate[fig-app-eval-41b.tex]{
		loglog
		--title 'Inferred \LTLf{} formula size'
		--xlabel '\SATDT{}' --ylabel '\MaxSATDT{}($\minscore=0.80$)'
		--table joinedByTraces.csv
		--columns LTL_size_SATDT:LTL_size_MaxSATDT80
		--min=1 --max=250
	}
\end{subfigure}

\begin{subfigure}{.45\linewidth}
	\centering
	\includepgfgenerate[fig-app-eval-41c.tex]{
		loglog
		--title 'Running time in $s$'
		--xlabel '\SATDT{}' --ylabel '\MaxSATDT{}($\minscore=0.60$)'
		--table joinedByTraces.csv
		--columns runtime_SATDT:runtime_MaxSATDT60
		--min=1e-3 %--max=1e3
	}
\end{subfigure}
%\hspace{1.5cm}
\begin{subfigure}{.45\linewidth}
	\centering
	\includepgfgenerate[fig-app-eval-41d.tex]{
		loglog
		--title 'Inferred \LTLf{} formula size'
		--xlabel '\SATDT{}' --ylabel '\MaxSATDT{}($\minscore=0.60$)'
		--table joinedByTraces.csv
		--columns LTL_size_SATDT:LTL_size_MaxSATDT60
		--min=1 --max=250
	}
\end{subfigure}

\caption{
	Comparison on all benchmarks of the performances of \MaxSATDT{}($\minscore$) and \SATDT{},
	with $\thres=0.05$ for both algorithms.
	$900 s$ of running time means that the algorithm timed out.
}
\label{app:fig:satdt-vs-maxsatdt}
\end{figure*}

\clearpage
\section{List of all the \LTL{} patterns used}
\label{app:sec:LTL-patterns}

We present in table \ref{tab:LTL-patterns:full} the exhaustive list of \LTL{} patterns we used to generate the benchmarks.

% Tab:PATTERNS
\begin{table}[h]
	\caption{Common \LTL{} patterns used in practice \cite{10.1145/298595.298598}}
	\label{tab:LTL-patterns:full}
	\resizebox{\linewidth}{!}{%
		\begin{tabular}{cccc}
			\hline
			Absence &
			Existence &
			Universality &
			Disjunction of common patterns
			\\ \hline
			$\lglobally( \lnot p_0)$ & % G(!(x0))
			$\leventually( p_0 )$ & % F(x0)
			$\lglobally( p_0 )$ & % G(x0)
			$\lglobally( \lnot p_0) \lor \leventually( p_0 \land \leventually( p_1 ) ) \lor
			\lglobally( \lnot p_3) \lor \leventually( p_2 \land \leventually( p_3 ) )$ % |(|(G(!(x0)),F(&(x0, F(x1)))), |(G(!(x3)),F(&(x2, F(x3)))))
			\\
			$\leventually(p_1) \limplies ( \lnot p_0 \luntil p_1 )$ & % ->(F(x1), U(!(x0),x1))
			$\lglobally( \lnot p_0) \lor \leventually( p_0 \land \leventually( p_1 ) )$ & % |(G(!(x0)),F(&(x0, F(x1))))
			$\leventually( p_1 ) \limplies ( p_0 \luntil p_1 )$ & % ->(F(x1), U(x0, x1))
			$\leventually( p_2 ) \lor \leventually( p_0 ) \lor \leventually( p_1 )$ % |(F(x2), |(F(x0), F(x1)))
			\\
			$\lglobally( p_1 \limplies \lglobally( \lnot p_0 ) )$ & % G(->(x1, G(!(x0))))
			$\lglobally( p_0 \land ( \lnot p_1 \limplies ( \lnot p_1 \luntil ( p_2 \land \lnot p_1 ) ) ) )$ & % G(&(x0,->(!(x1),U(!(x1),&(x2, !(x1))))))
			$\lglobally( p_1 \limplies \lglobally( p_0 ) )$ & % G(->(x1, G(x0)))
			$\lglobally( p_0 \land ( \lnot p_1 \limplies ( \lnot p_1 \luntil ( p_2 \land \lnot p_1 ) ) ) ) \lor
			\lglobally( p_3 \land ( \lnot p_4 \limplies ( \lnot p_4 \luntil ( p_5 \land \lnot p_4 ) ) ) )$ % |(G(&(x0,->(!(x1),U(!(x1),&(x2, !(x1)))))), G(&(x3,->(!(x4),U(!(x4),&(x5, !(x4)))))))
			\\ \hline
	\end{tabular}}
\end{table}
